# Supplementary material for: Measurement of the $t\bar{t}Z$ and $t\bar{t}W$ production cross sections in multilepton final states using 3.2 fb$^{-1}$ of $pp$ collisions at $\sqrt{s}$ = 13 TeV with the ATLAS detector
Source: arXiv:1609.01599 source file (2017-02-06)
Supplement: Supplementary file 1 [file appendix.tex]

\part*{Auxiliary material}

\begin{figure}[hb!]
\includegraphics[width=0.8\linewidth]{Ranking_TTZ_final.pdf}                
\caption{\label{fig:ranking_ttZData} The fitted values of the nuisance
parameters for the most important sources of systematic uncertainty and their
impact on the measured signal strength $\mu$, for the \ttZ fit. The points, which are
drawn conforming to the scale of the bottom axis, show the deviation of each of
the fitted nuisance parameters, $\theta$, from $\theta_0$, which is the nominal
value of that nuisance parameter, in units of the pre-fit standard deviation
$\Delta\theta$. The error bars show the post-fit uncertainties,
$\sigma_\theta$, which are close to 1 if the data do not provide any further
constraint on that uncertainty. Conversely, a value of $\sigma_\theta$ much
smaller than 1 indicates a significant reduction with respect to the original
uncertainty. The nuisance parameters are sorted according to their post-fit
effect on $\mu$ (blue areas), conforming to the scale of the top axis, with
those with the largest impact at the top. }
\end{figure}

\begin{figure}
\includegraphics[width=0.8\linewidth]{Ranking_TTW_final.pdf}                
\caption{\label{fig:ranking_ttWData} 
The fitted values of the nuisance parameters for the most important sources of
systematic uncertainty and their impact on the measured signal strength $\mu$, for
the \ttW fit. The points, which are drawn conforming to the scale of the bottom
axis, show the deviation of each of the fitted nuisance parameters, $\theta$,
from $\theta_0$, which is the nominal value of that nuisance parameter, in
units of the pre-fit standard deviation $\Delta\theta$.  For the WZ
normalisation factor, the fitted value of the normalisation parameter, which has
a pre-fit value of one, is shown together with its uncertainties.  The error
bars show the post-fit uncertainties, $\sigma_\theta$, which are close to 1 if
the data do not provide any further constraint on that uncertainty. Conversely,
a value of $\sigma_\theta$ much smaller than 1 indicates a significant
reduction with respect to the original uncertainty. The nuisance parameters are
sorted according to their post-fit effect on $\mu$ (blue areas), conforming to
the scale of the top axis, with those with the largest impact at the top.}
\end{figure}

\begin{table}[htbp]
\centering 
\caption{Event yields after the fit for signal and backgrounds,
and the observed data in all control and signal regions used in the fit to
extract the \ttZ and \ttW cross sections.  The quoted uncertainties in the
event yields represent statistical and systematic uncertainties.
The \tZ, \WtZ, \ttH, three- and four-top-quark processes are
denoted $t+X$. The $WZ$, $ZZ$, $H \to ZZ$ (ggF and VBF), $HW$ and $HZ$ and VBS
processes are denoted `Bosons'.
\vspace{1ex}}

\resizebox{\columnwidth}{!}{
\begin{tabular}{%
c|
r@{\,}@{$\pm$}@{\,}l
r@{\,}@{$\pm$}@{\,}l
r@{\,}@{$\pm$}@{\,}l
r@{\,}@{$\pm$}@{\,}l
|r@{\,}@{$\pm$}@{\,}l
r@{\,}@{$\pm$}@{\,}l
|r
}
\toprule
Region &
\multicolumn{2}{c}{$t+X$} &
\multicolumn{2}{c}{Bosons} &
\multicolumn{2}{c}{Fake leptons} &
\multicolumn{2}{c|}{Total bkg.} &
\multicolumn{2}{c}{\ttW} &
\multicolumn{2}{c|}{\ttZ} &
Data \\
\midrule
\TLCR&   $0.51$ & $0.13$&        $29$ & $6$&     $2.1$ & $1.8$&          $31$ & $7$&     $0.037$ & $0.023$&      $0.88$ & $0.32$&        33\\
\FLCR&   \multicolumn{2}{c}{$<0.001$} &          $37$ & $7$&     $1.8$ & $0.6$&          $39$ & $7$&     \multicolumn{2}{c}{$<0.001$} &          $0.028$ & $0.012$&      39\\
\midrule
\SSLSR&          $0.93$ & $0.09$&        $0.13$ & $0.07$&        $1.4$ & $1.2$&          $2.5$ & $1.3$&          $5.8$ & $3.0$&          $0.76$ & $0.26$&        9\\
\TLSRC&          $1.07$ & $0.25$&        $0.6$ & $0.5$&          \multicolumn{2}{c}{$<0.001$} &          $1.6$ & $0.5$&          $0.16$ & $0.09$&        $6.0$ & $2.0$&          8\\
\TLSRA&          $1.12$ & $0.24$&        $2.7$ & $1.6$&          $2.1$ & $1.7$&          $5.8$ & $2.4$&          $0.09$ & $0.05$&        $4.7$ & $1.6$&          7\\
\TLSRB&          $0.58$ & $0.19$&        $0.25$ & $0.21$&        \multicolumn{2}{c}{$<0.001$} &          $0.82$ & $0.28$&        $0.21$ & $0.11$&        $2.1$ & $0.7$&          4\\
\TLSRD&          $0.96$ & $0.11$&        $0.15$ & $0.14$&        $3.3$ & $2.2$&          $4.5$ & $2.2$&          $4.0$ & $2.1$&          $1.6$ & $0.5$&          10\\
\FLSRD&          $0.212$ & $0.033$&      $0.08$ & $0.06$&        $0.113$ & $0.022$&      $0.40$ & $0.08$&        \multicolumn{2}{c}{$<0.001$} &          $0.72$ & $0.25$&        1\\
\FLSRE&          $0.121$ & $0.022$&      $0.07$ & $0.06$&        $0.062$ & $0.012$&      $0.25$ & $0.07$&        \multicolumn{2}{c}{$<0.001$} &          $0.69$ & $0.23$&        1\\
\FLSRB&          $0.25$ & $0.04$&        $0.0131$ & $0.0032$&    $0.114$ & $0.019$&      $0.37$ & $0.04$&        \multicolumn{2}{c}{$<0.001$} &          $0.82$ & $0.28$&        2\\
\FLSRC&          $0.16$ & $0.05$&        \multicolumn{2}{c}{$<0.001$} &          $0.063$ & $0.013$&      $0.23$ & $0.05$&        \multicolumn{2}{c}{$<0.001$} &          $0.70$ & $0.23$&        1\\
\bottomrule
\end{tabular}
}
\end{table}
